# Supplementary material for: TorchRL: A data-driven decision-making library for PyTorch
Source: arXiv:2306.00577 source file (2023-11-27)
Supplement: Supplementary file 1 [file Appendix.tex]

\documentclass{article}

% if you need to pass options to natbib, use, e.g.:
%     \PassOptionsToPackage{numbers, compress}{natbib}
% before loading neurips_2023

% ready for submission
\usepackage[preprint]{neurips_2023}

% to compile a preprint version, e.g., for submission to arXiv, add add the
% [preprint] option:
%     \usepackage[preprint]{neurips_2023}

% to compile a camera-ready version, add the [final] option, e.g.:
%     \usepackage[final]{neurips_2023}

% to avoid loading the natbib package, add option nonatbib:
%    \usepackage[nonatbib]{neurips_2023}

\usepackage[utf8]{inputenc} % allow utf-8 input
\usepackage[T1]{fontenc}    % use 8-bit T1 fonts
\usepackage{hyperref}       % hyperlinks
\usepackage{url}            % simple URL typesetting
\usepackage{booktabs}       % professional-quality tables
\usepackage{amsfonts}       % blackboard math symbols
\usepackage{nicefrac}       % compact symbols for 1/2, etc.
\usepackage{microtype}      % microtypography
\usepackage{xcolor}         % colors
\usepackage{listings}
\usepackage{subcaption}
\usepackage{enumitem}
\usepackage{float}
\setlist{leftmargin=2mm}
\usepackage[pdftex]{graphicx}
\usepackage{subcaption}
\usepackage[export]{adjustbox}
\usepackage[title]{appendix}
\lstset{escapeinside={<@}{@>}}
\usepackage{pythonhighlight}
\usepackage{threeparttable}
\definecolor{myred}{RGB}{255,0,0}
\definecolor{mygreen}{RGB}{0,255,0}

\definecolor{codegreen}{rgb}{0,0.6,0}
\definecolor{othergreen}{rgb}{0.31,0.98,0.48}
\definecolor{codegray}{rgb}{0.5,0.5,0.5}
\definecolor{codepurple}{rgb}{0.58,0,0.82}
\definecolor{backcolour}{rgb}{0.157,0.165,0.21}
\definecolor{basic}{rgb}{0.97,0.97,0.95}

\lstdefinestyle{mystyle}{
    backgroundcolor=\color{backcolour},   
    commentstyle=\color{othergreen},
    keywordstyle=\color{magenta},
    numberstyle=\tiny\color{codegray},
    stringstyle=\color{codegreen},
    basicstyle={\small,\color{basic}},
    breakatwhitespace=false,         
    breaklines=true,                 
    captionpos=b,                    
    keepspaces=true,                 
    numbers=left,                    
    numbersep=5pt,                  
    showspaces=false,                
    showstringspaces=false,
    showtabs=false,                  
    tabsize=2
}
\lstset{style=mystyle}

\title{TorchRL: Appendix}

\begin{document}

\maketitle

\input{appendix_content}

\bibliographystyle{unsrt}
\bibliography{bibliography}

\end{document}
