# Supplementary material for: TorchRL: A data-driven decision-making library for PyTorch
Source: arXiv:2306.00577 source file (2023-11-27)
Supplement: Supplementary file 2 [file env_wrappers.tex]

\subsection{Transforms}
At present, TorchRL encompasses a diverse array of transformations, each designed to alter, include, or add different aspects of a TensorDict. The transformations range from refining image inputs through resizing, cropping, and normalization procedures, to manipulating reward structures via binarization and scaling.
In addition, TorchRL's collection of transformations includes more general functions, such as the ability to unsqueeze, introduce noise, stack, or concatenate objects within a TensorDict.
This comprehensive selection of transformations offers users the flexibility to adapt and optimize their TorchRL implementations according to their specific needs and objectives.
